# Supplementary material for: L*ReLU: Piece-wise Linear Activation Functions for Deep Fine-grained Visual Categorization
Source: arXiv:1910.12259 source file (2019-10-27)
Supplement: Supplementary file 1 [file supplementary.tex]

\begin{figure*}[!hb]
\centering
    	\begin{subfigure}{0.33\textwidth}
        	\centering
        	\includegraphics[page=6, width=\textwidth]{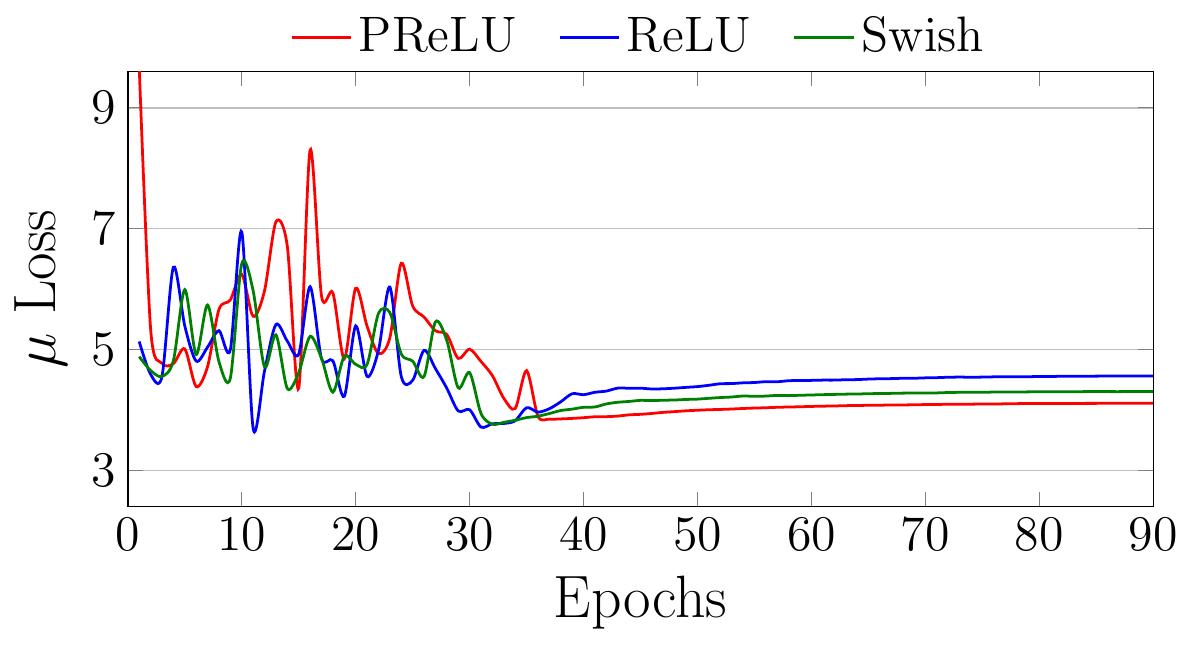}
        	\caption{Car Dataset}
            %	\caption{Coarse-grained datasets: mean and standard deviation for all datasets and AFs.}
    	\end{subfigure}%
        	\begin{subfigure}{0.33\textwidth}
        	\centering
        	\includegraphics[page=7, width=\textwidth]{results/Loss_Result.pdf}
        	\caption{Food Dataset}
            %	\caption{Coarse-grained datasets: mean and standard deviation for all datasets and AFs.}
    	\end{subfigure}%
    	%\hfill
        \begin{subfigure}{0.33\textwidth}
        	\centering
        	\includegraphics[page=9, width=\textwidth]{results/Loss_Result.pdf}
        	\caption{Bird Dataset}
            %	\caption{Coarse-grained datasets: mean and standard deviation for all datasets and AFs.}
        \end{subfigure}
    	\begin{subfigure}{0.33\textwidth}
        	\centering
        	\includegraphics[page=10,, width=\textwidth]{results/Loss_Result.pdf}
        	\caption{Aircraft Dataset}
            %	\caption{Coarse-grained datasets: mean and standard deviation for all datasets and AFs.}
    	\end{subfigure}%
    	\begin{subfigure}{0.33\textwidth}
        	\centering
        	\includegraphics[page=8, width=\textwidth]{results/Loss_Result.pdf}
        	\caption{Dog Dataset}
            %	\caption{Coarse-grained datasets: mean and standard deviation for all datasets and AFs.}
    	\end{subfigure}%
\caption{Average of Categorical Cross-Entropy Loss Train over three runs }
\label{fig:losses}
\end {figure*}

\prmk{How much effort would it be to add other losses? \mbrmk{it takes time if it is really necessary I can add it but I think is not crucial} For us, in particular for you it is clear why Swish is shown, but this might not be the case for many potential reviewers ...}

\subsection{Convergence}

Finally, we would also like to show that the proper choice of the activation function also influences the convergence behaviour of the networks. Thus, in Figure\\ref{fig:losses}, we plot the training losses over 90 epochs for \relu, \prelu, and \swish for all five datasets. In particular, it can be seen (as expected) that \prelu allows for a faster convergence compared to \relu, in particular for the more complex datasets. Moreover, the convergence speed is comparable to \swish. \prmk{Would we like to say something like that?}
